# Supplementary material for: DESI Strong Lens Foundry I: HST Observations and Modeling with GIGA-Lens
Source: arXiv:2502.03455 source file (2025-02-06)
Supplement: Supplementary file 1 [file appendix_complete_cornerplot.tex]

\subsection*{B. Full corner plot}

\vspace{8 pt}
\begin{minipage}{\linewidth}
\makebox[\linewidth]{
  \includegraphics[keepaspectratio=true,scale=0.09]{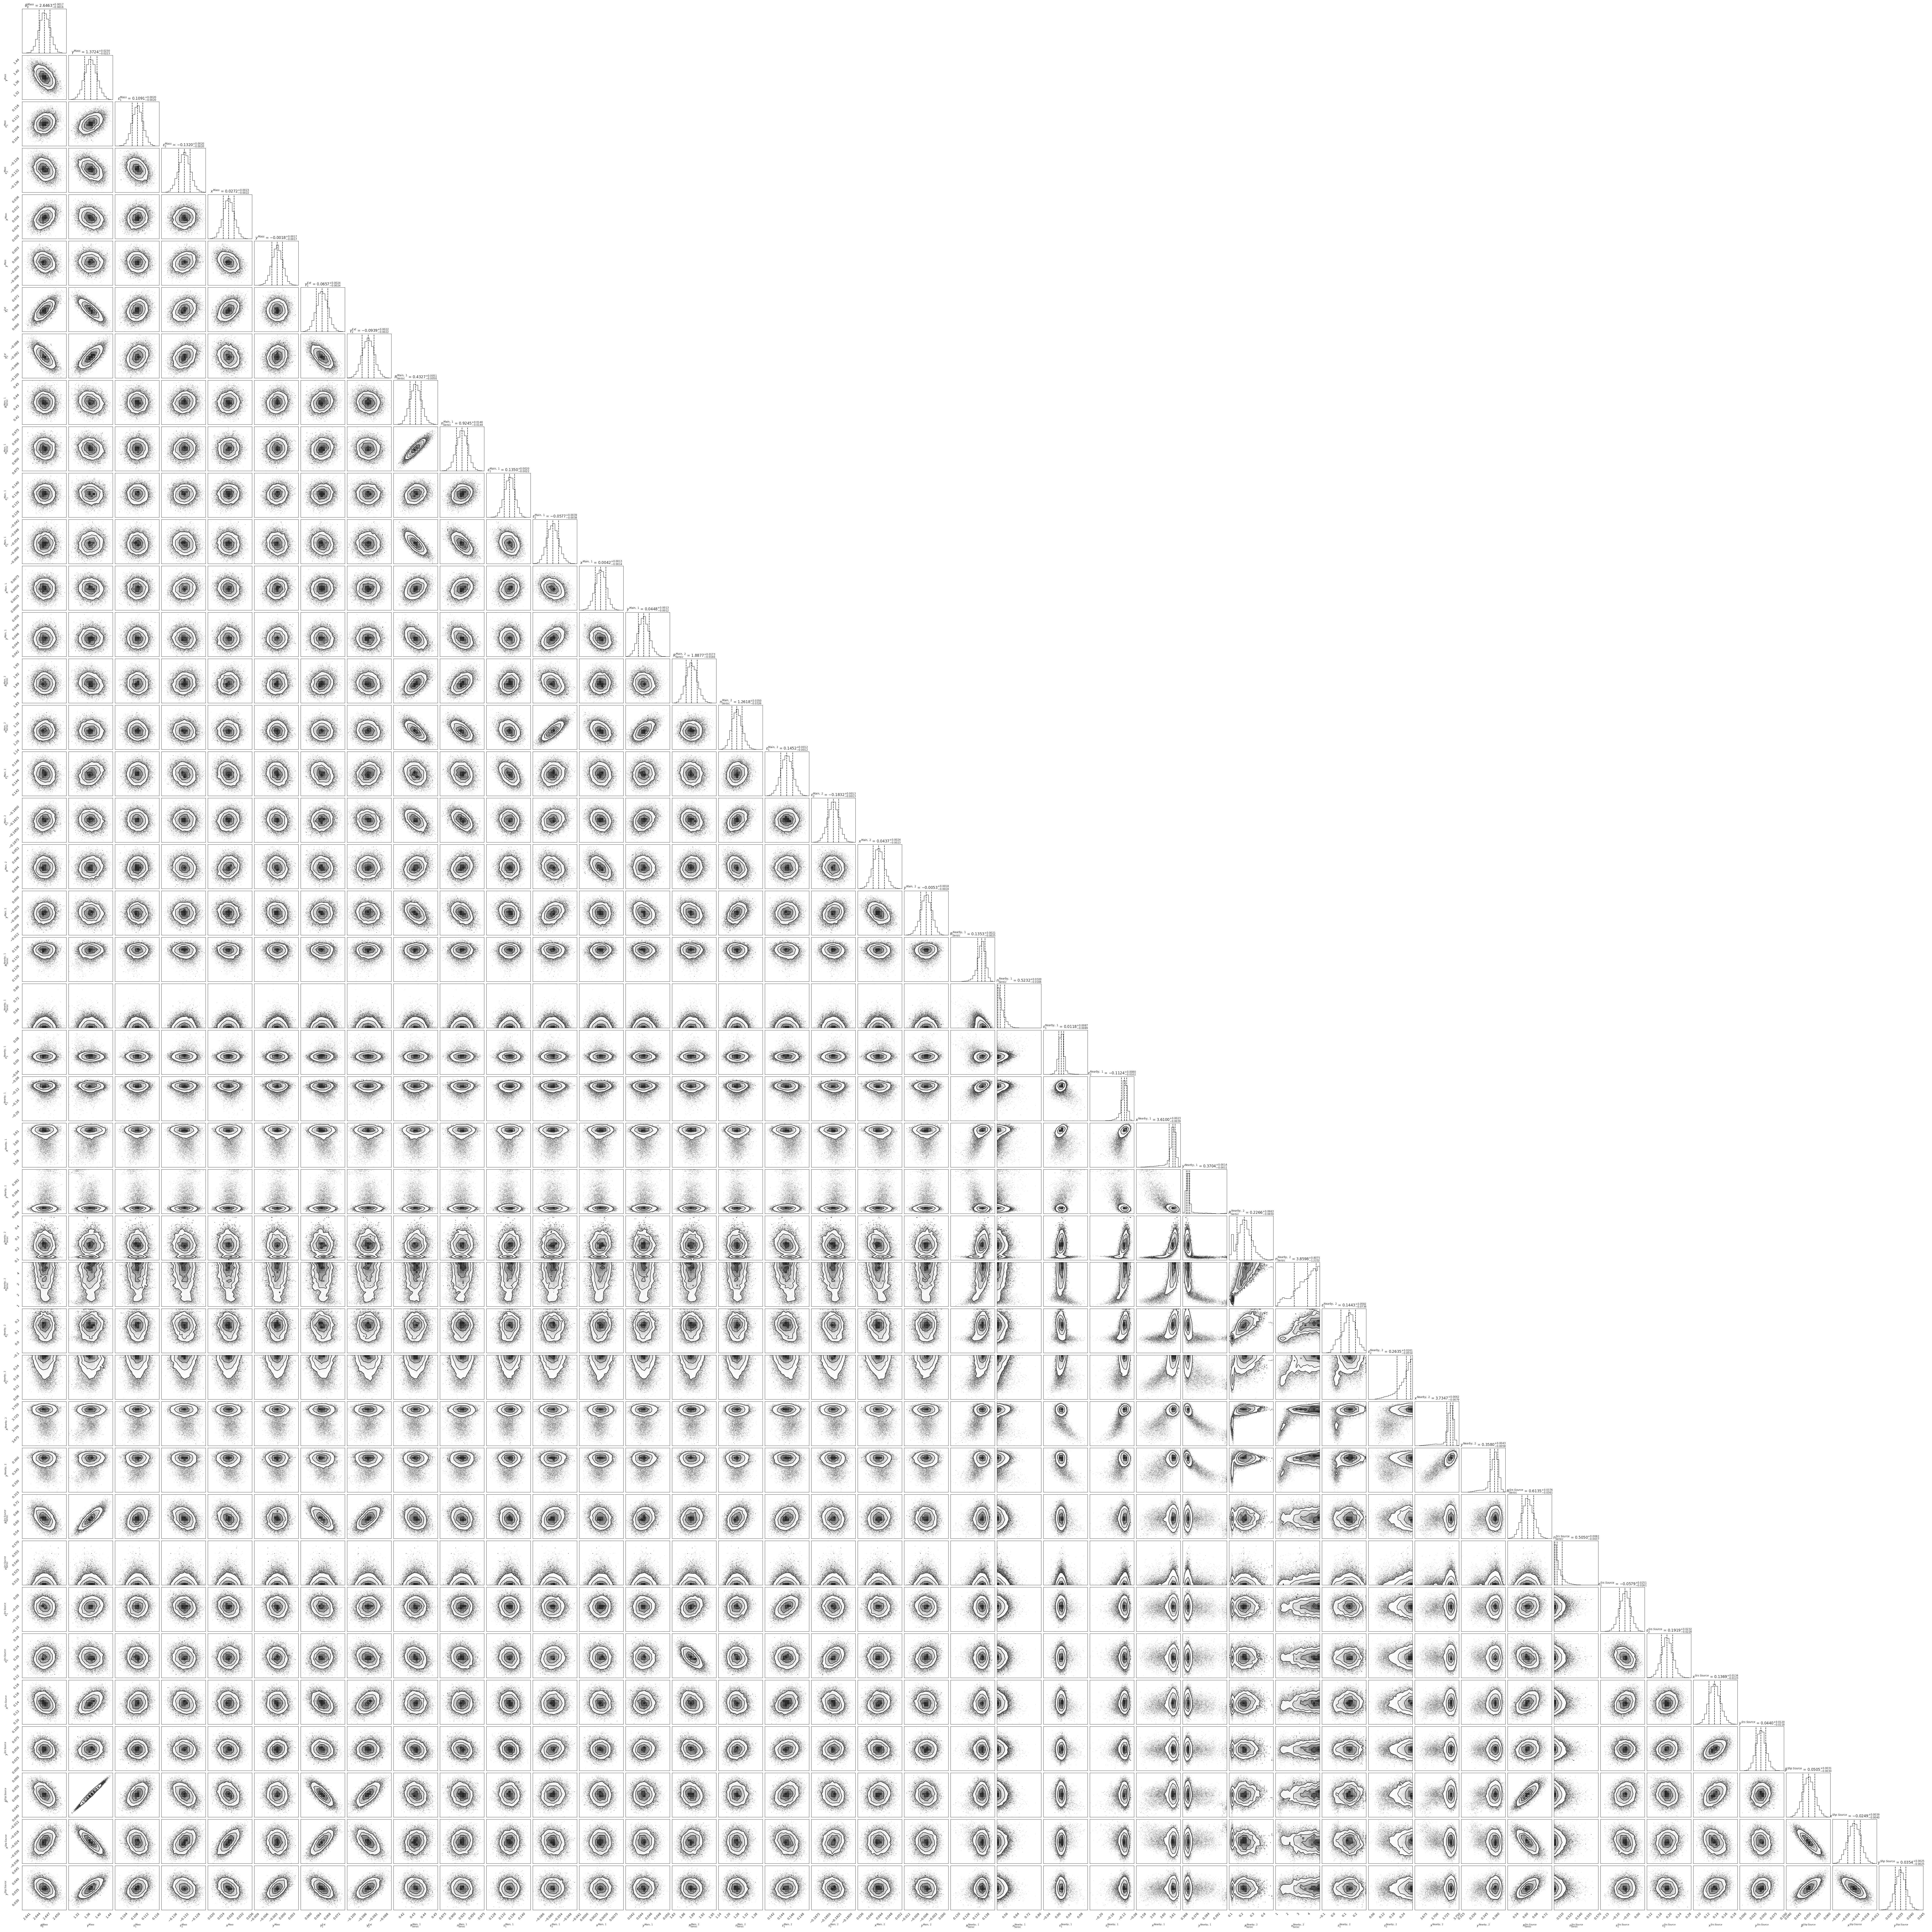}}
\captionof{figure}{The corner plot shows our sampling results for all 41 parameters of our model. The superscripts represent the system's object each parameter belong to. Therefore, \textit{Mass} refers to the lens mass profile, which is an EPL and \textit{Ext} to the external shear. \textit{Main, 1} and \textit{Main, 2} each denote one of the elliptical S{\'e}rsic profiles that comprise the lens light. Equivalently, \textit{Nearby, 1} and \textit{Nearby, 2} describe the two elliptical S{\'e}rsic profiles of the nearby galaxy. Lastly, \textit{Srs Source} and \textit{Shp Source} account for the elliptical S{\'e}rsic component and the Shapelets component of the source, respectively.
The subscripts provide further description for the parameter if necessary. $\theta_E$ is the Einstein radius of the lens mass profile. $\epsilon_1$ and $\epsilon_2$ are the eccentricities of the respective profile, EPL or elliptical S{\'e}rsic, depending on the superscript. $\gamma_1$ and $\gamma_2$ are the external shear components. $R_{Sersic}$ and $n_{Sersic}$ are the half-light radius and the S{\'e}rsic index of the corresponding profile.
Note that the anomalies in this cornerplot are all related to the nearby galaxy but one, the S{\'e}rsic index for the source.
%Maybe elaborate on this
}

\label{fig:full_cornerplot}
\end{minipage}
